# Supplementary material for: Chirally Factorised Truncated Conformal Space Approach
Source: arXiv:2201.06509 ancillary file (2022-05-05)
Supplement: Supplementary file 1 [file CFTCSA_PackageContents.pdf]

## CFTCSA package description

The ancillary file package includes the various data files, Matlab functions and example codes.

To run the example codes, the ancillary file package must be downloaded and extracted into a folder. The only further step necessary is navigating to this folder, using `cd` command in terminal or adding the corresponding path to Matlab using the `'addpath'` command. Brief description of all functions is given in their header and can be accessed from Matlab using the `'help'` command.

The package contains:

- 4 example codes for concrete physical problems.
- 8 basic Matlab functions comprising the implementation of the CFTCSA.
- 3 directories containing the basic CFT data.

### Example codes

- CFTCSA\_e8\_spectrum.m: a Matlab *function* computing the lowest few energy levels of the  $E_8$  model.
- CFTCSA\_SG\_Spectrum.m: a Matlab *function* computing the lowest few energy levels of the sine-Gordon model.
- CFTCSA\_Tricrit\_FormFactors.m: a Matlab *function* computing the 1-particle Form Factors of the leading and subleading magnetisation operators for the 1st and 3rd particles in the  $E_7$  theory.
- SG\_TimeEvolution.m: a Matlab *script* which can be run from terminal or by using Matlab's interface and copy-pasting the lines. The script computes the time evolution of the cosine operator in the sine-Gordon theory when quenching from the ground state of the free compact boson CFT. The result of the time evolution is plotted and saved in a png file `'CosTPlot.png'`.

### Basic Matlab functions

- ImportMatFile.m: imports a `' .mat'` file consisting of a list of *sparse* matrices and produces and Matlab cell-list, whose elements are matrices of *sparse* format.
- ImportMatFileNoSparse.m: same as ImportMatFile, but the matrices in the `' .mat'` file and in the Matlab cell-list are non-sparse ones.
- VectorFromTensor.m: transforms a generic vector represented in terms of tensors to a conventional vector.
- TensorsFromVector.m: produces a vector represented in terms of *sparse* tensors from a standard vector.
- TensorsFromVectorNoSparse.m: same as TensorsFromVector, but with conventional, non-sparse tensors.
- ApplyOperator.m: implements the action of a (generic) scaling field on vectors.
- ApplyHamiltonian.m: implements the action of a (generic) Hamiltonian on vectors.
- TimeEvolutionChebyshev.m: implements the Chebyshev-Bessel time evolution of a generic vector.

## TCSA data

The 3 folders containing the required TCSA data in appropriate format are:

- IsingFieldTheory\_Data
- SG\_Data
- TricriticalIsing\_Data

These contain the various descriptors (Chiral Descriptors, Hilbert Space Descriptors, Operator Matrix Descriptors) in '.dat' format, the Operator Lists in '.mat' format and the Structure Constant Matrices in '.dat' format for the three different models considered in our work.

For the massless boson CFT, the scripts only use the perturbing operator  $\cos(\phi/R)$ , therefore the CFT data only contain the corresponding Operator Descriptor Matrix, Structure Constant Matrix and Operator List. Furthermore, since in this case the left and right Operator Descriptor Matrices are the same, only one such matrix is given.

For the Ising and tricritical Ising CFT, the scripts use more than one primary fields, listed below.

- The CFT data of the Ising model contain two scaling fields:
  - $\varepsilon$  (energy)
  - $\sigma$  (magnetisation)

requiring two sets of operator data (Operator Descriptor Matrix, Structure Constant Matrix and Operator List), which are distinguished by the words 'Eps' and 'Sig' in the names of the files. For each field, the left and right Operator Descriptor Matrices are given separately as indicated by the letters 'L' and 'R' in the file names.

- The CFT data of the tricritical Ising model contain five scaling fields:
  - $\varepsilon$  (energy)
  - $t$  (vacancy density)
  - $\varepsilon''$  (sub-leading energy field)
  - $\sigma$  (magnetisation)
  - $\sigma'$  (subleading magnetisation)

requiring five sets of operator data (Operator Descriptor Matrix, Structure Constant Matrix and Operator List), which are distinguished by the words 'Eps', 'T', 'EpsPPrime', 'Sig' and 'SigPrime' in the names of the files. For each field, the left and right Operator Descriptor Matrices are given separately as indicated by the letters 'L' and 'R' in the file names.
